# Supplementary material for: ShapeGlot: Learning Language for Shape Differentiation
Source: arXiv:1905.02925 source file (2019-05-08)
Supplement: Supplementary file 1 [file out_of_dist_listening_with_attention.tex]

%!TEX root = ../../sections/main.tex
\begin{table*}[t!]
\caption{Transfer-learning of neural listeners in {\em unseen object classes}. The evaluating listener is trained with chair data uses word-attention but not point-clouds. In each row the listener's accuracy is reported for a given shape-net class in different sub-populations of the transfer data. {\bf entire}: entire transfer dataset, {\bf known}: utterances of which all the words are in the training-vocabulary, {\bf with part}: subset of {\bf known} utterances that contain at least one part-related, {\bf without part}: subset of {\bf known} with zero part-related words. The listener uses word attention but not point-clouds. (Average accuracies over five random seeds controlling the training, and the data-splits are displayed).}
\label{table:ood_human_listening_with_attn}

\begin{tabular}{|l||r|r|r|r|r|}
\hline
\backslashbox{Population}{\begin{tabular}{@{}c@{}}Class\end{tabular}} &  bed  &  chair  & lamp  &  sofa & table\\
\hline
entire       & 54.5 $\pm 3.3\%$       &  77.5  $\pm 0.9\%$      &  50.6 $\pm 2.1\%$         &  53.7 $\pm 2.0\%$ &  64.0 $\pm 0.8\%$\\

\hline
known        & 54.7 $\pm 3.7\%$       & 77.8 $\pm 0.9\%$        &  52.7 $\pm 1.5\%$         &  55.0 $\pm 2.8\%$ &  65.9 $\pm 1.2\%$\\

\hline
with part    & {\bf 60.3} $\pm 3.6\%$ & 77.0 $\pm1.0\%$         & {\bf 58.4} $\pm  2.8\%$   & 54.9 $\pm 3.5\%$ &  {\bf 67.9} $\pm 2.1\%$\\

\hline
without part & 51.7 $\pm 4.5\%$      &  {\bf 80.8} $\pm 0.9\%$ & 49.6 $\pm 2.4\%$           &  {\bf 55.3} $\pm 4.0\%$ &  63.9 $\pm 1.3\%$\\
\hline
\end{tabular}
\end{table*}
